# Supplementary material for: Visual Alignment Constraint for Continuous Sign Language Recognition
Source: arXiv:2104.02330 source file (2021-08-18)

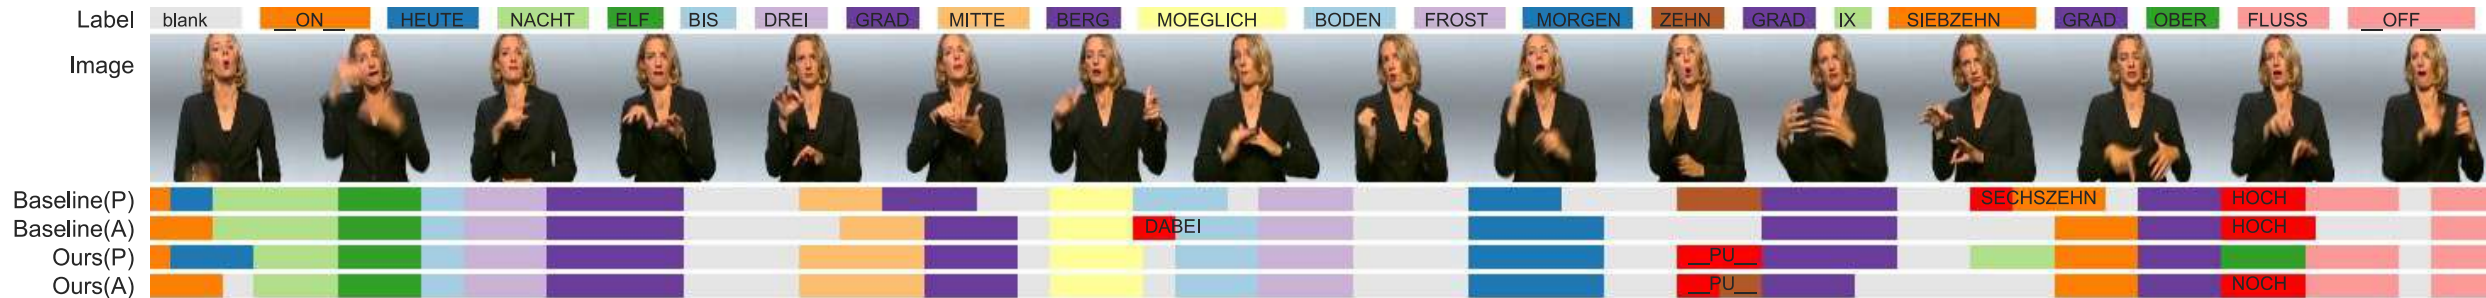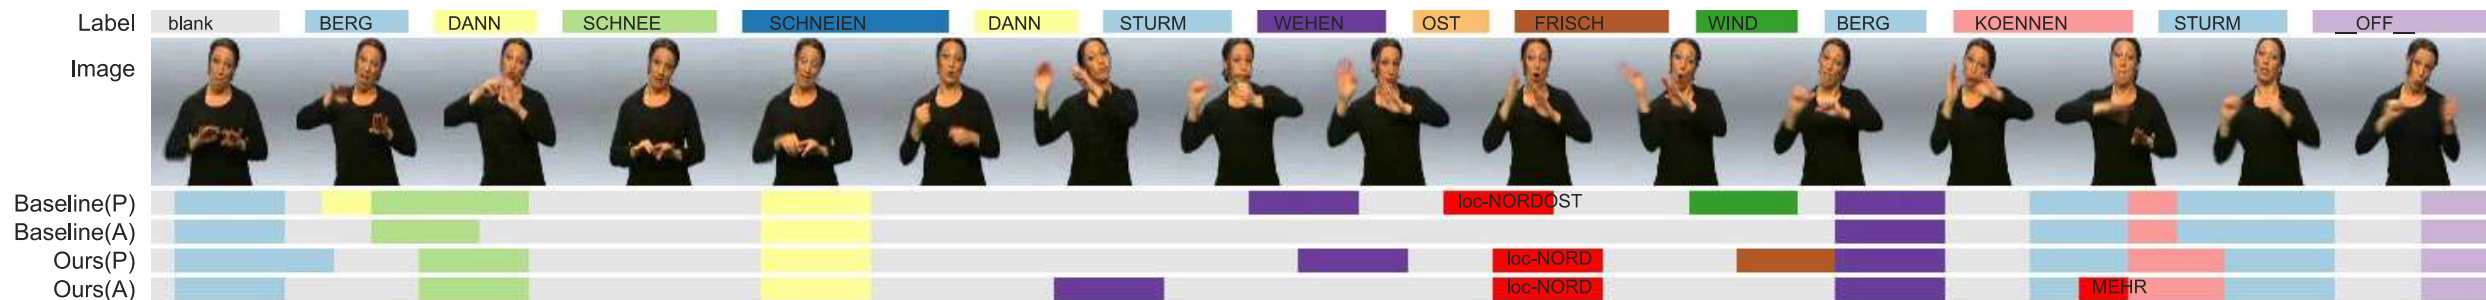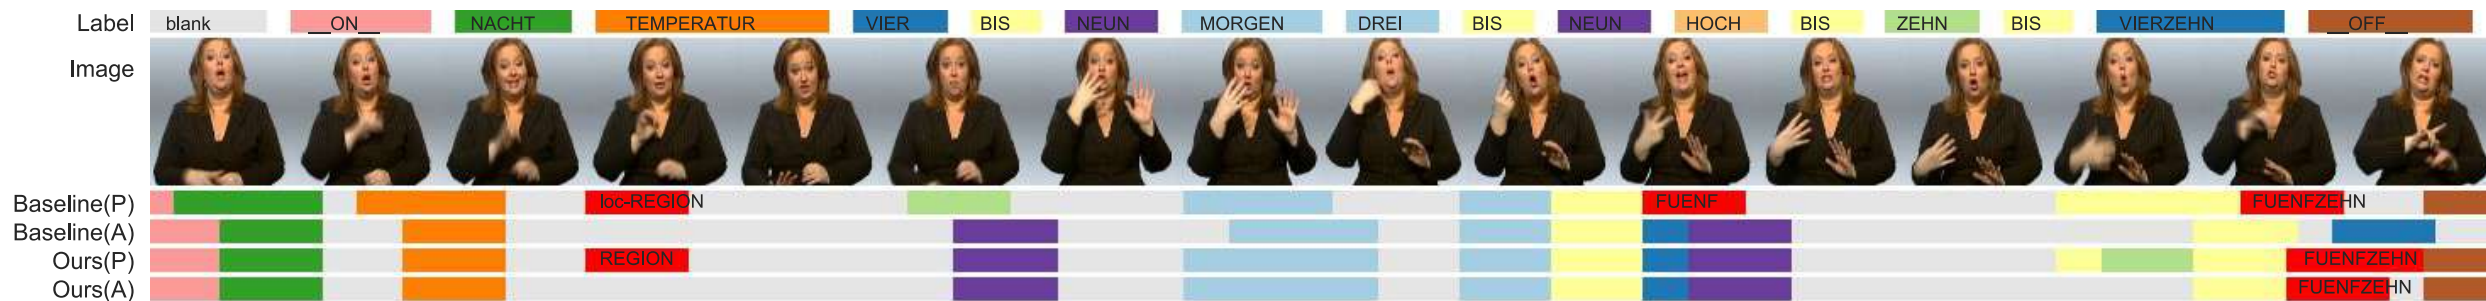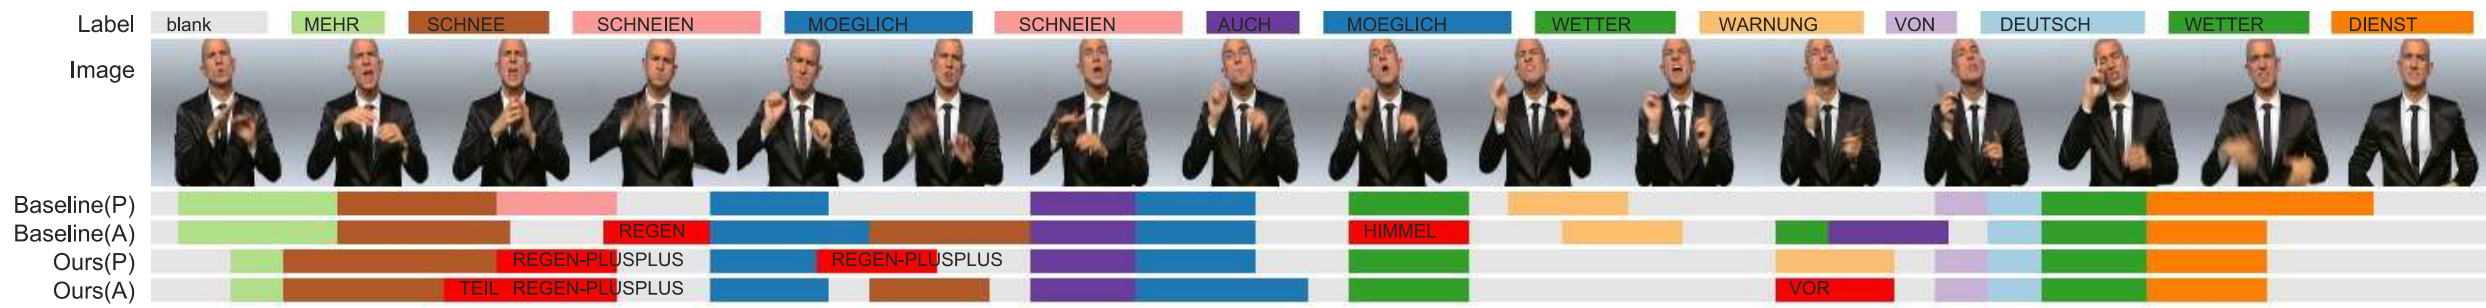

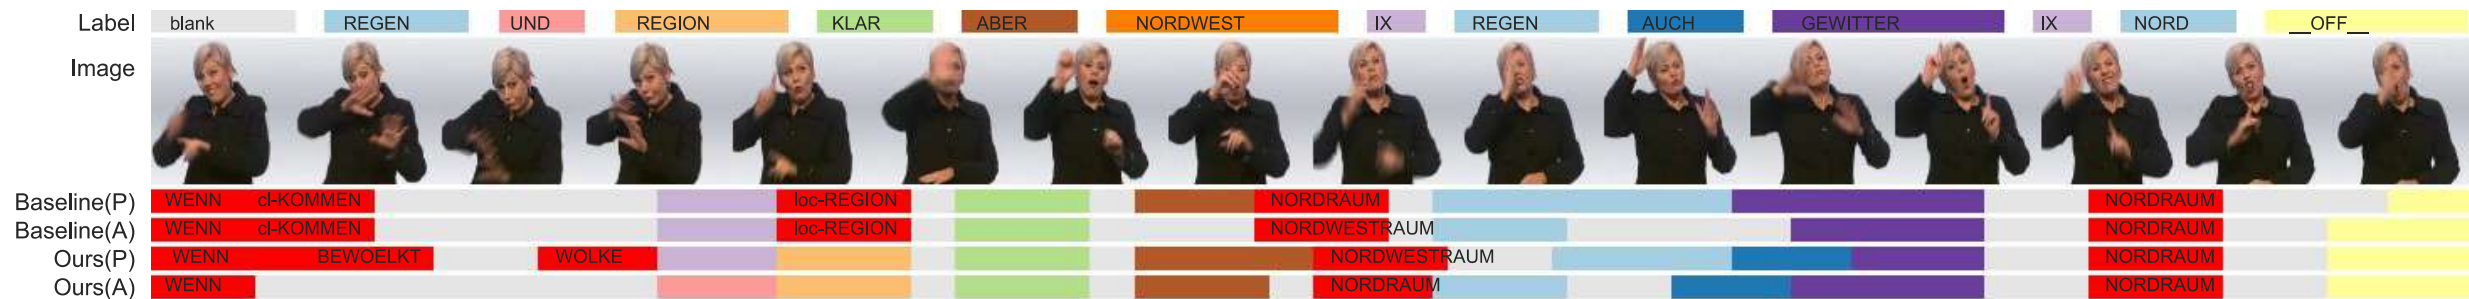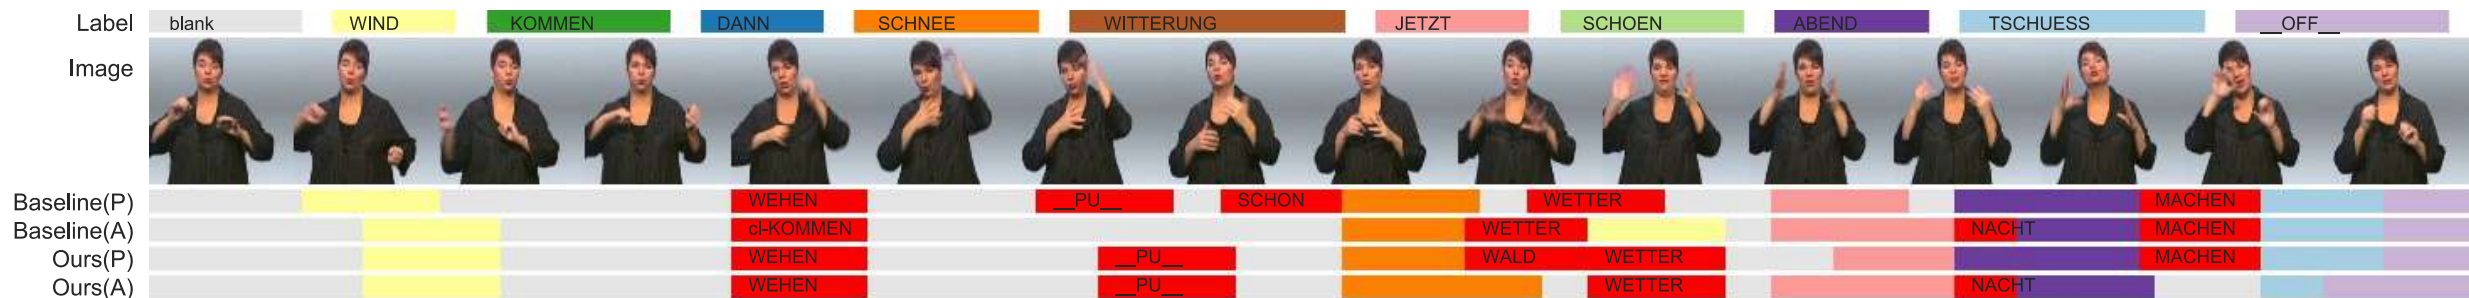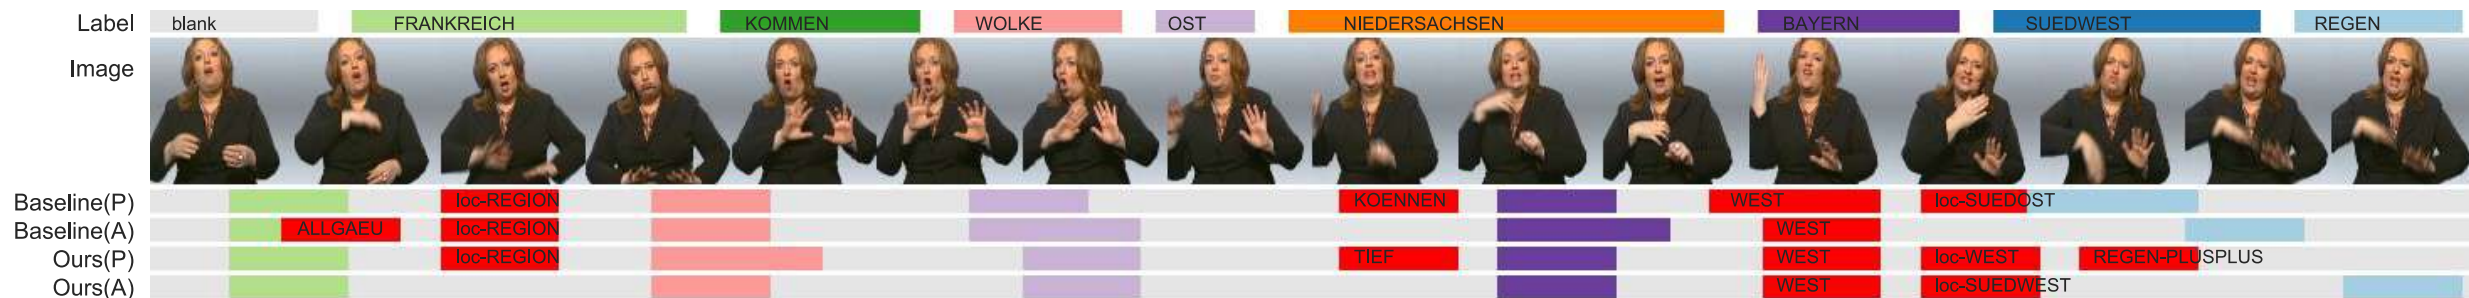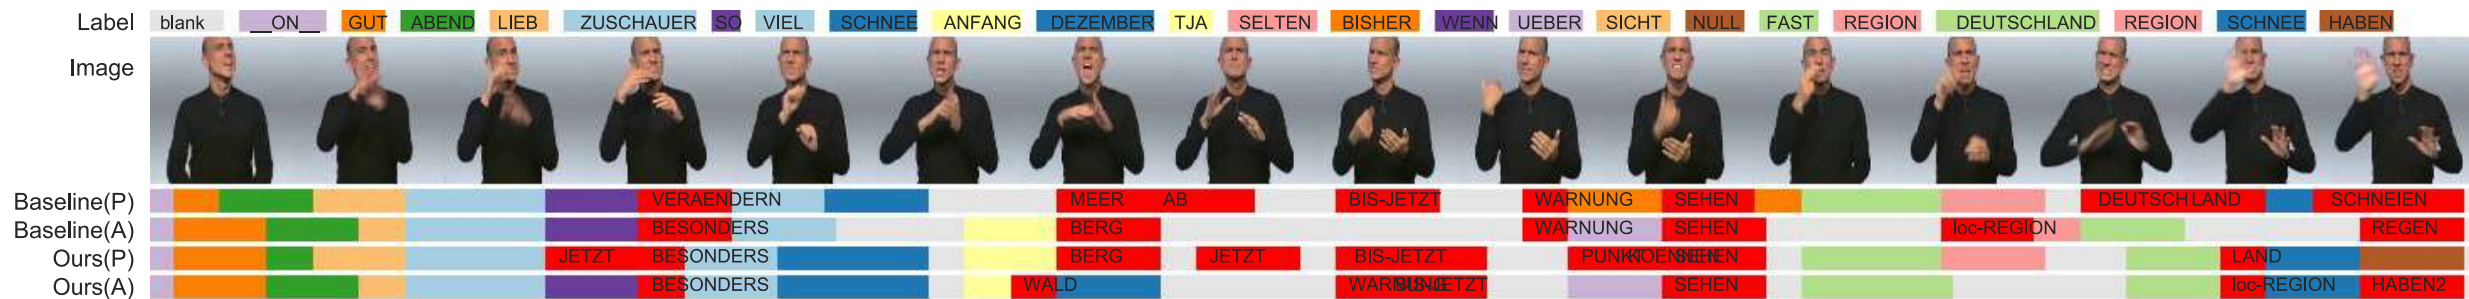

Supplement: Supplementary file 1 [file supp_figure12_visual.pdf]
