# Supplementary material for: Visual Alignment Constraint for Continuous Sign Language Recognition
Source: arXiv:2104.02330 source file (2021-08-18)
Supplement: Supplementary file 2 [file supp_figure9_compare.pdf]

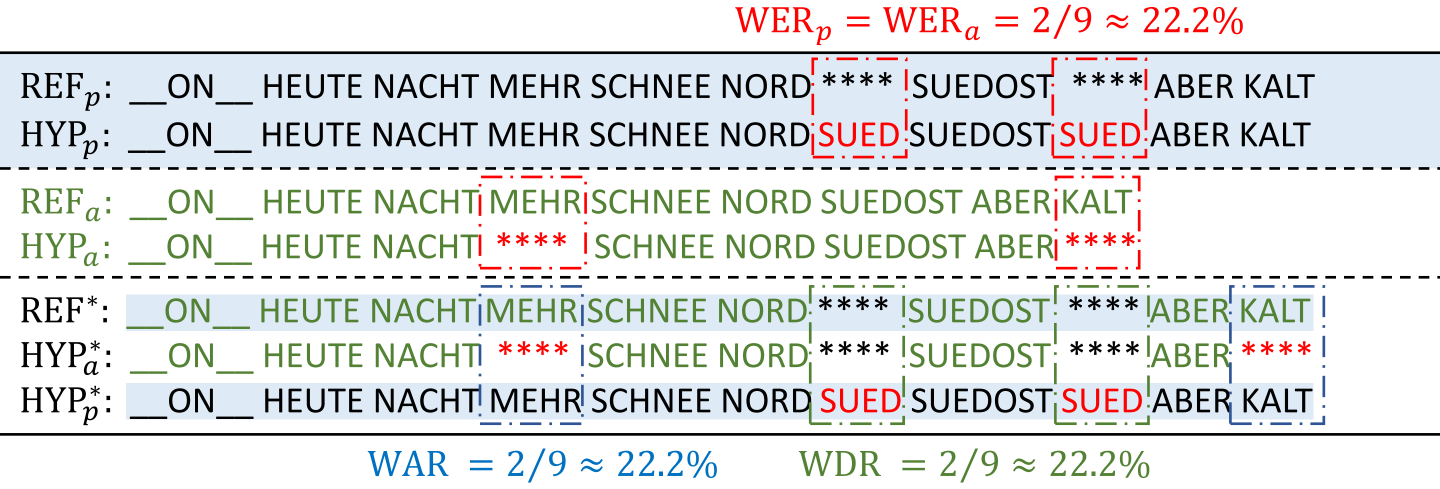

WER_p = WER_a = 2/9 ≈ 22.2%
REF_p: __ON__ HEUTE NACHT MEHR SCHNEE NORD **** SUEDOST **** ABER KALT
HYP_p: __ON__ HEUTE NACHT MEHR SCHNEE NORD SUED SUEDOST SUED ABER KALT
REF_a: __ON__ HEUTE NACHT MEHR SCHNEE NORD SUEDOST ABER KALT
HYP_a: __ON__ HEUTE NACHT **** SCHNEE NORD SUEDOST ABER ****
REF*: __ON__ HEUTE NACHT MEHR SCHNEE NORD **** SUEDOST **** ABER KALT
HYP*_a: __ON__ HEUTE NACHT **** SCHNEE NORD **** SUEDOST **** ABER ****
HYP*_p: __ON__ HEUTE NACHT MEHR SCHNEE NORD SUED SUEDOST SUED ABER KALT
WAR = 2/9 ≈ 22.2%
WDR = 2/9 ≈ 22.2%

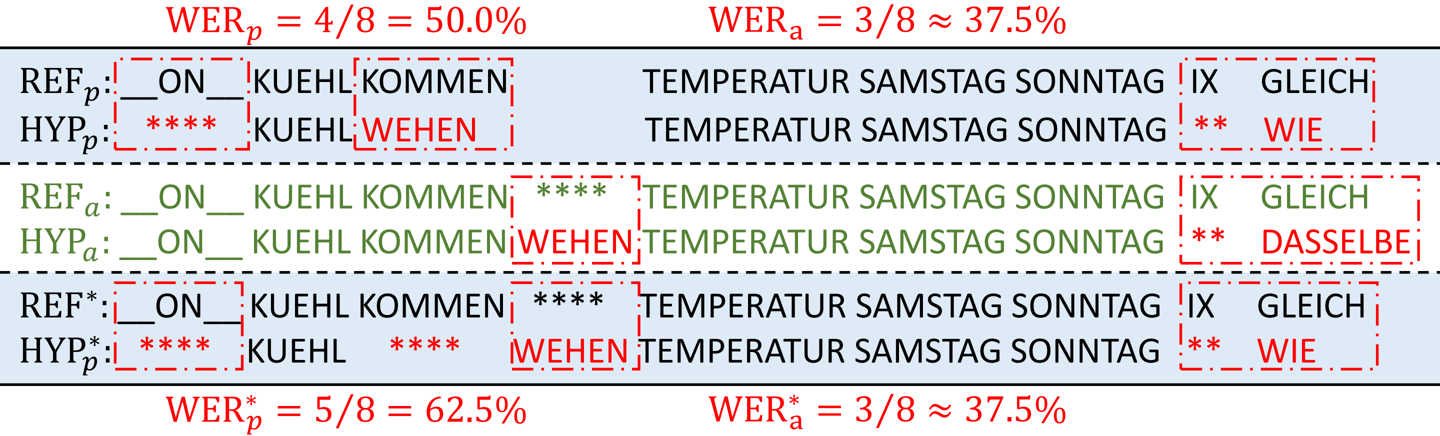

WER_p = 4/8 = 50.0%
WER_a = 3/8 ≈ 37.5%
REF_p: __ON__ KUEHL KOMMEN TEMPERATUR SAMSTAG SONNTAG IX GLEICH
HYP_p: **** KUEHL WEHEN TEMPERATUR SAMSTAG SONNTAG ** WIE
REF_a: __ON__ KUEHL KOMMEN **** TEMPERATUR SAMSTAG SONNTAG IX GLEICH
HYP_a: __ON__ KUEHL KOMMEN WEHEN TEMPERATUR SAMSTAG SONNTAG ** DASSELBE
REF*: __ON__ KUEHL KOMMEN **** TEMPERATUR SAMSTAG SONNTAG IX GLEICH
HYP*_p: **** KUEHL **** WEHEN TEMPERATUR SAMSTAG SONNTAG ** WIE
WER*_p = 5/8 = 62.5%
WER*_a = 3/8 ≈ 37.5%

$\mathrm{WER}_p = 2/8 = 25.0\%$ $\mathrm{WER}_\mathrm{a} = 2/8 = 25.0\%$

$\mathrm{REF}_p$: MORGEN BESONDERS NORD REGION UND **** WEST **** REGEN KOENNEN

$\mathrm{HYP}_p$: MORGEN BESONDERS NORD REGION UND WEST WEST DANN REGEN KOENNEN

$\mathrm{REF}_a$: MORGEN BESONDERS NORD REGION UND WEST REGEN KOENNEN

$\mathrm{HYP}_a$: MORGEN BESONDERS NORD NACHT WEST WEST REGEN KOENNEN

$\mathrm{REF}^*$: MORGEN BESONDERS NORD REGION UND **** WEST **** REGEN KOENNEN

$\mathrm{HYP}_a^*$: MORGEN BESONDERS NORD **** *** NACHT WEST WEST REGEN KOENNEN

$\mathrm{WER}_p^* = 2/8 = 25.0\%$ $\mathrm{WER}_\mathrm{a}^* = 4/8 = 50.0\%$
