# Supplementary material for: Visual Alignment Constraint for Continuous Sign Language Recognition
Source: arXiv:2104.02330 source file (2021-08-18)

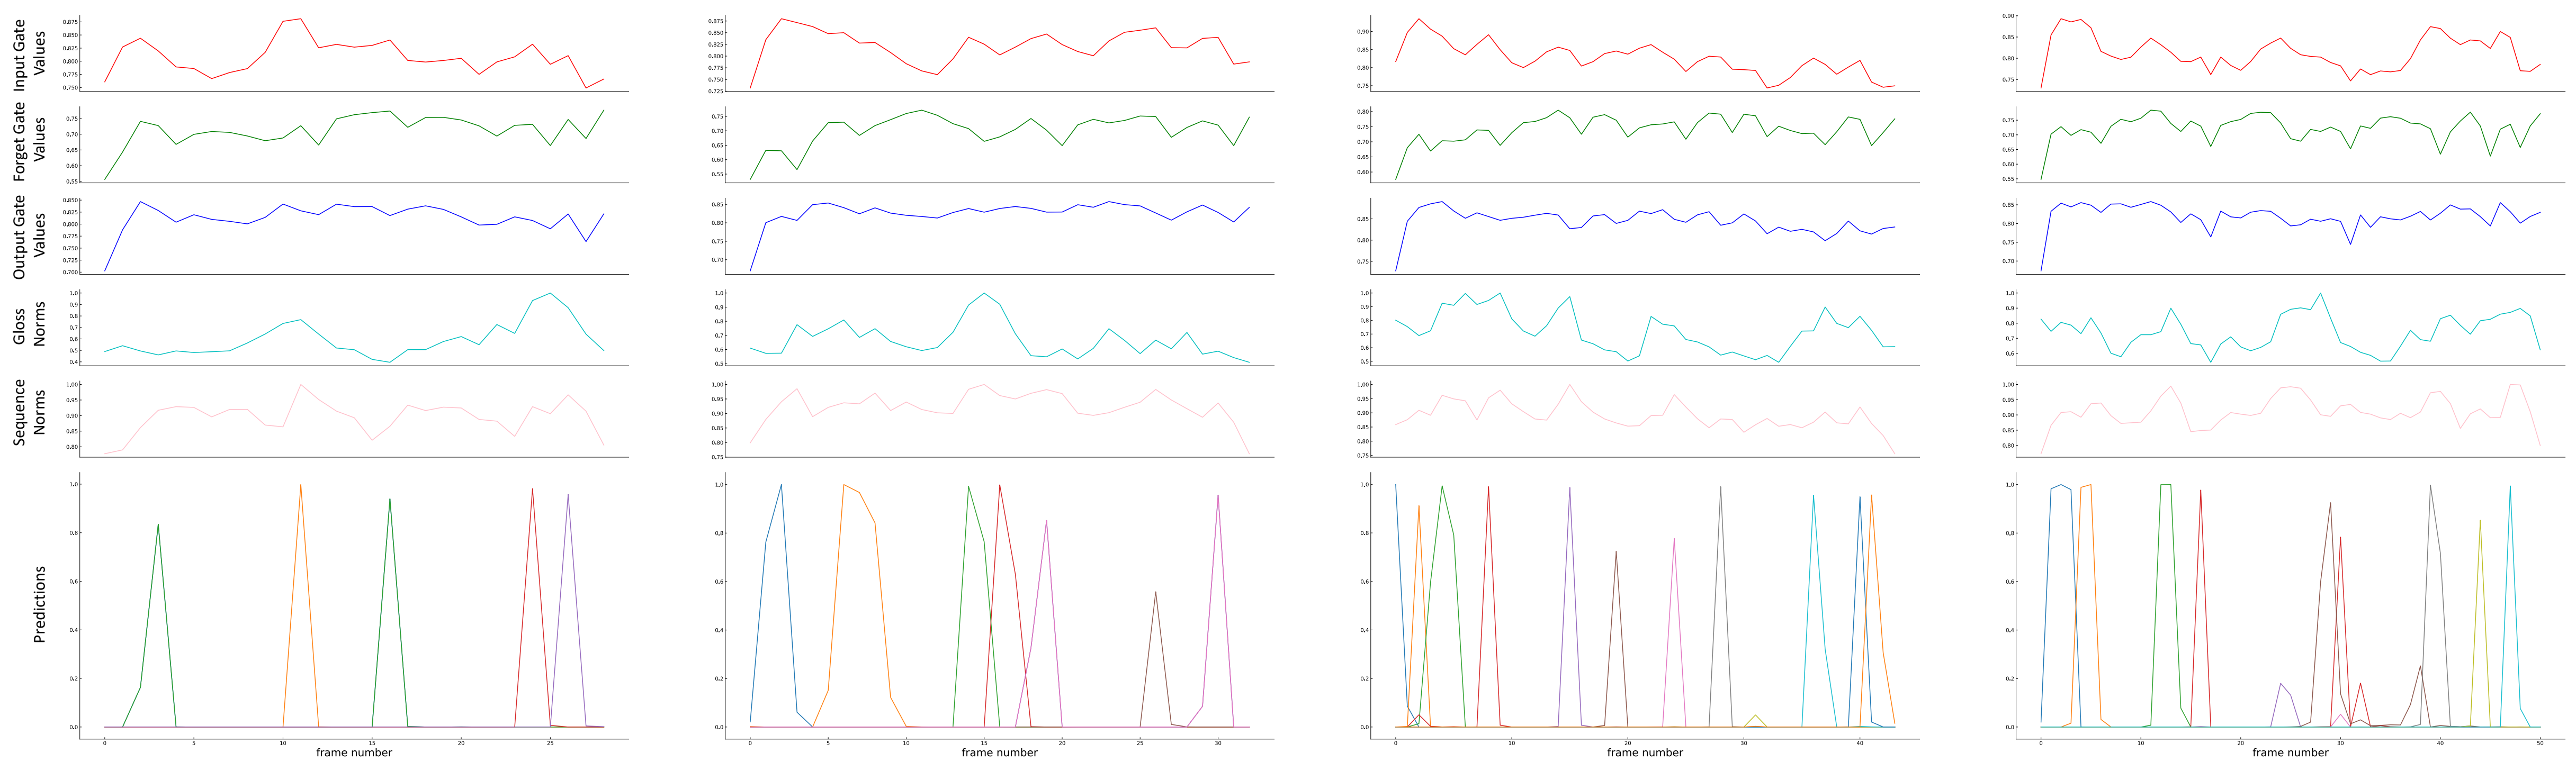

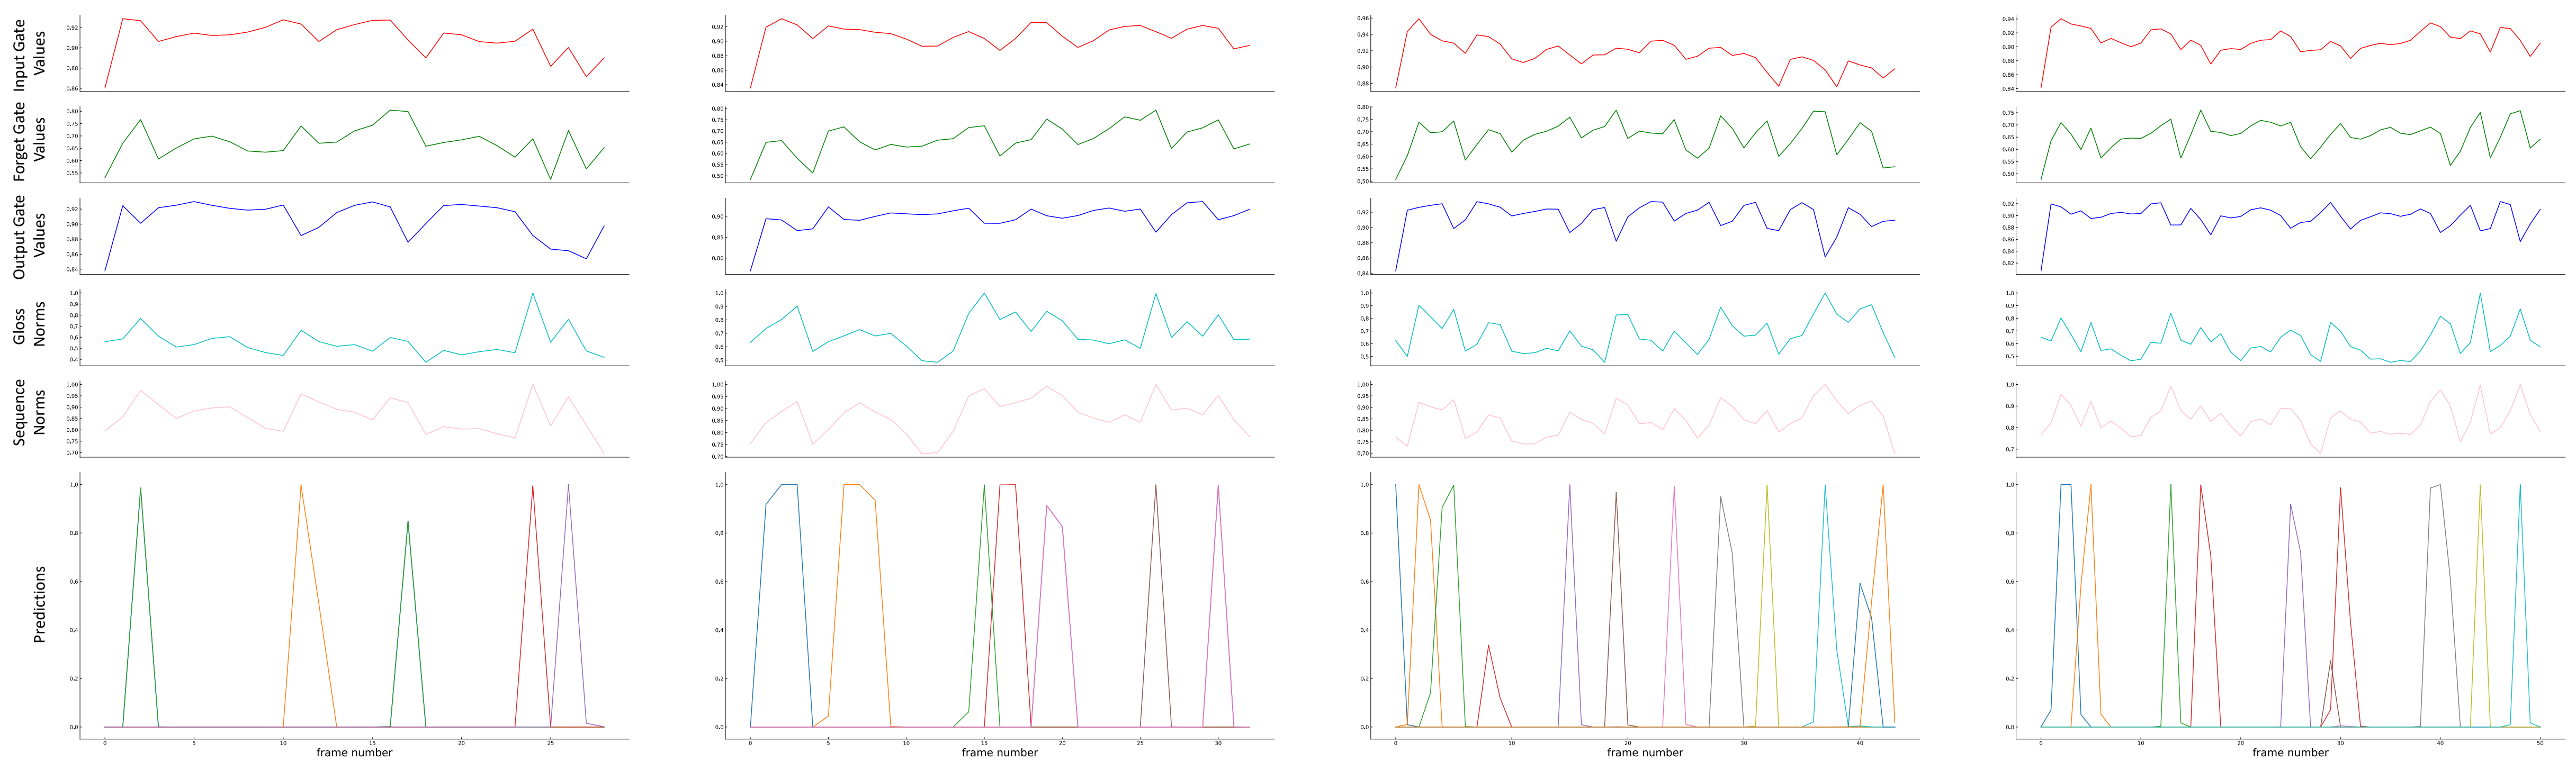

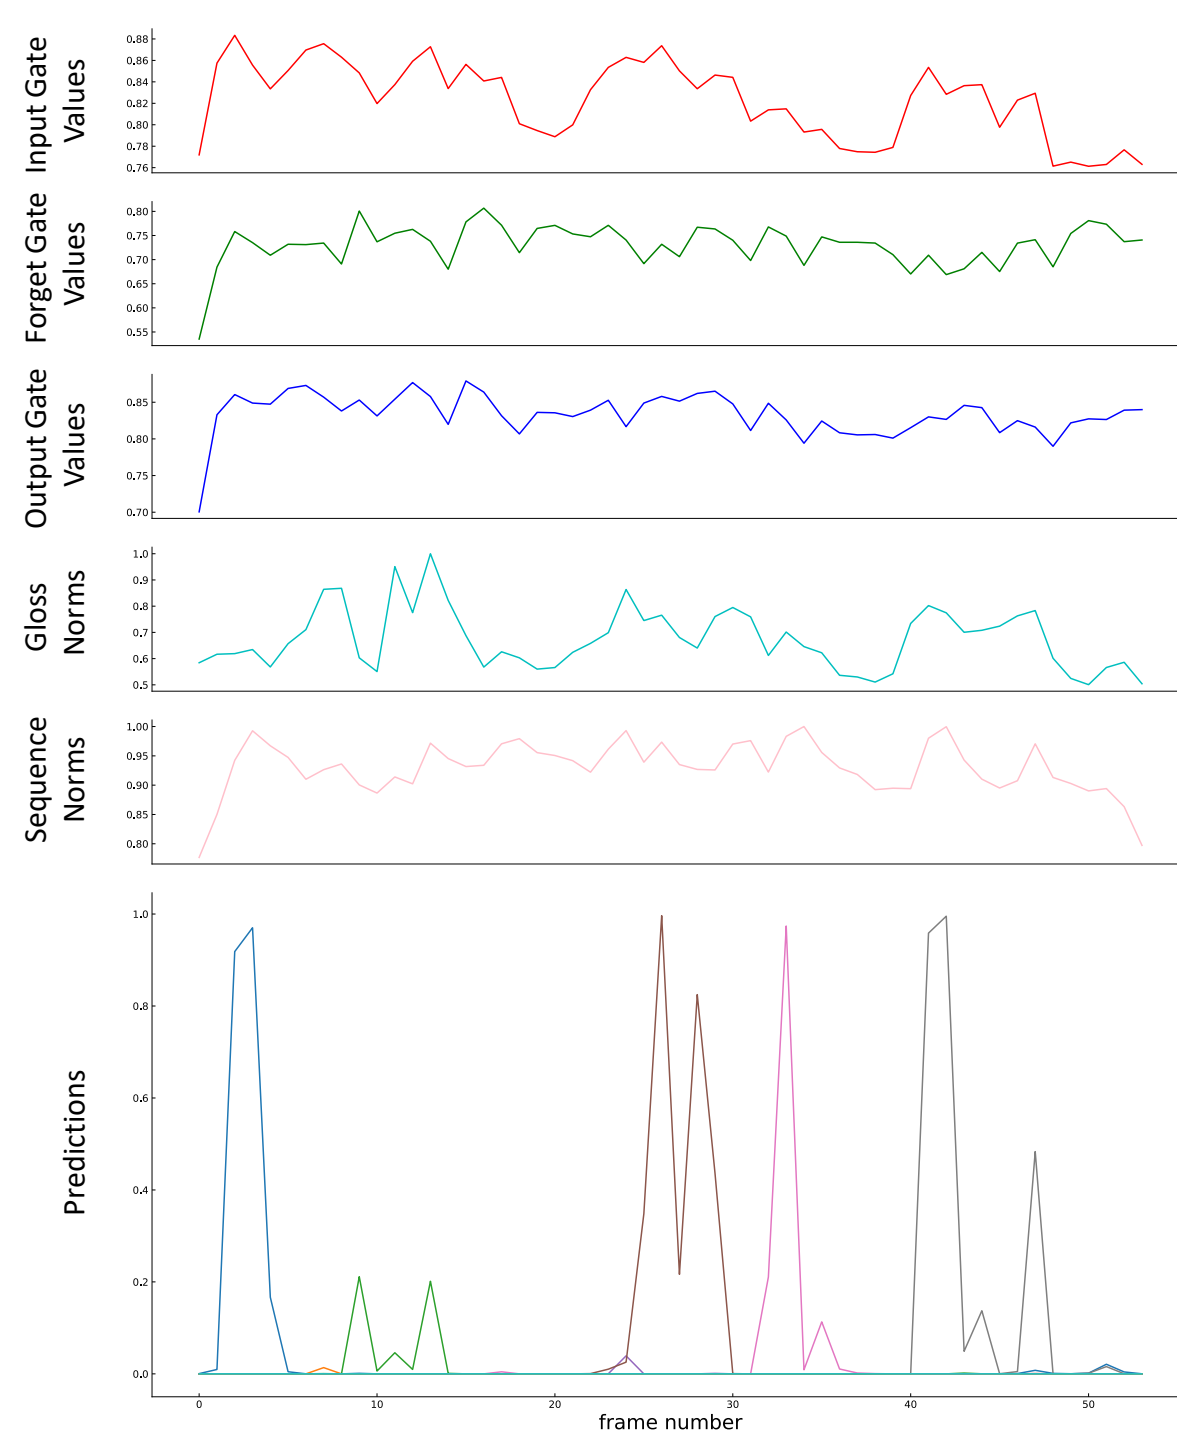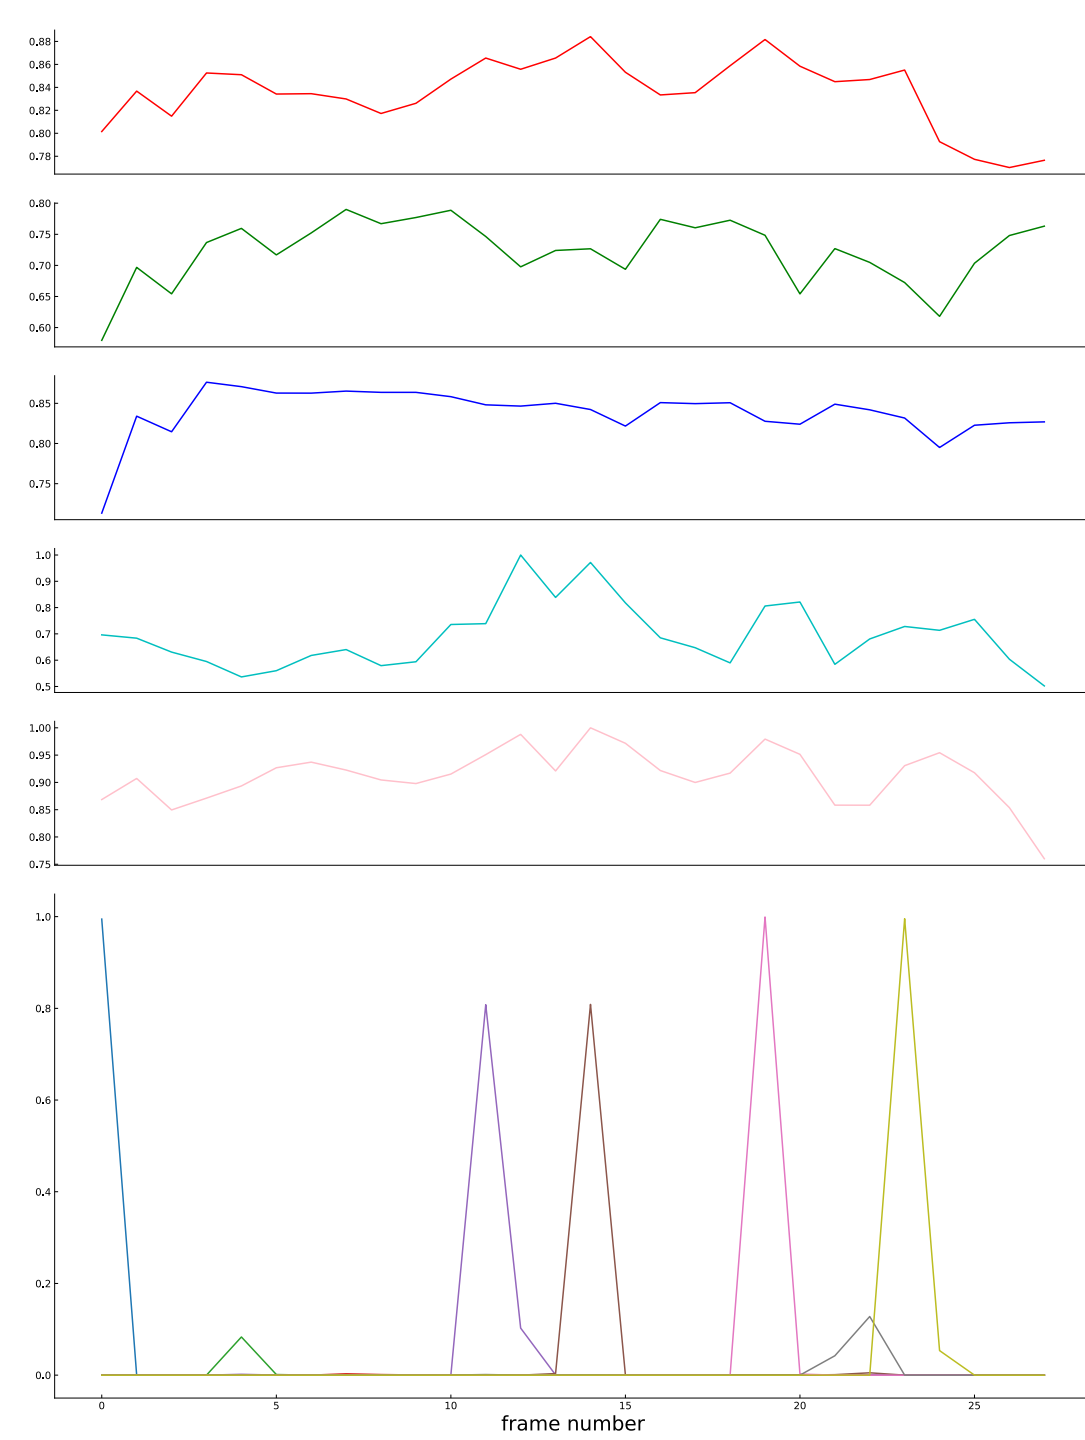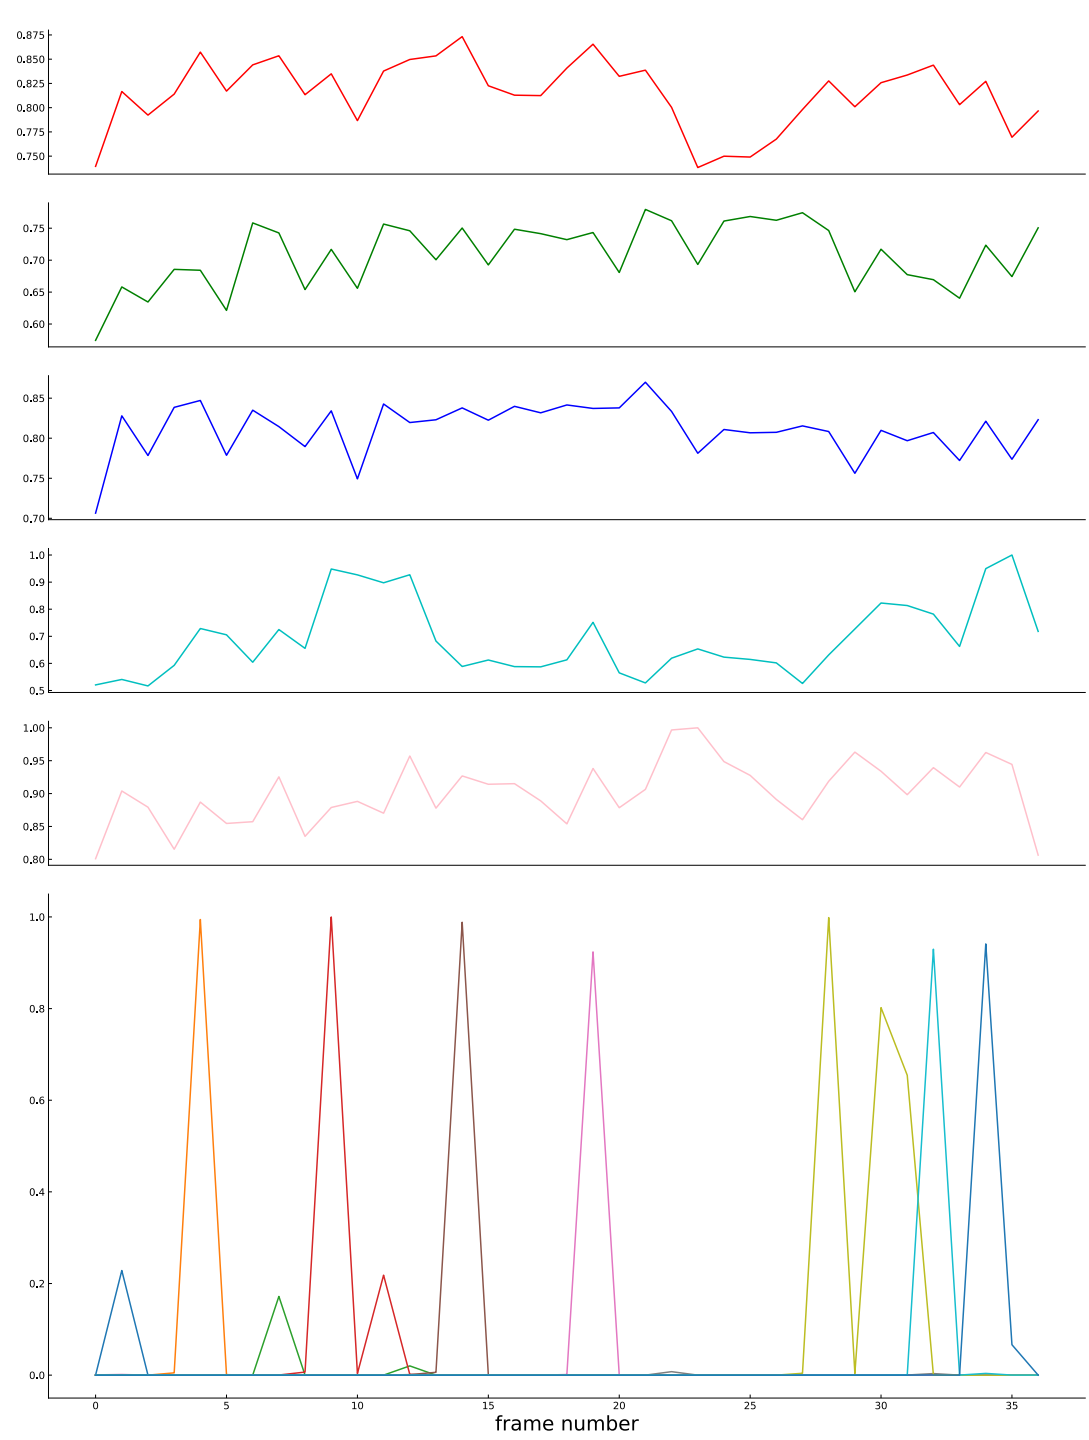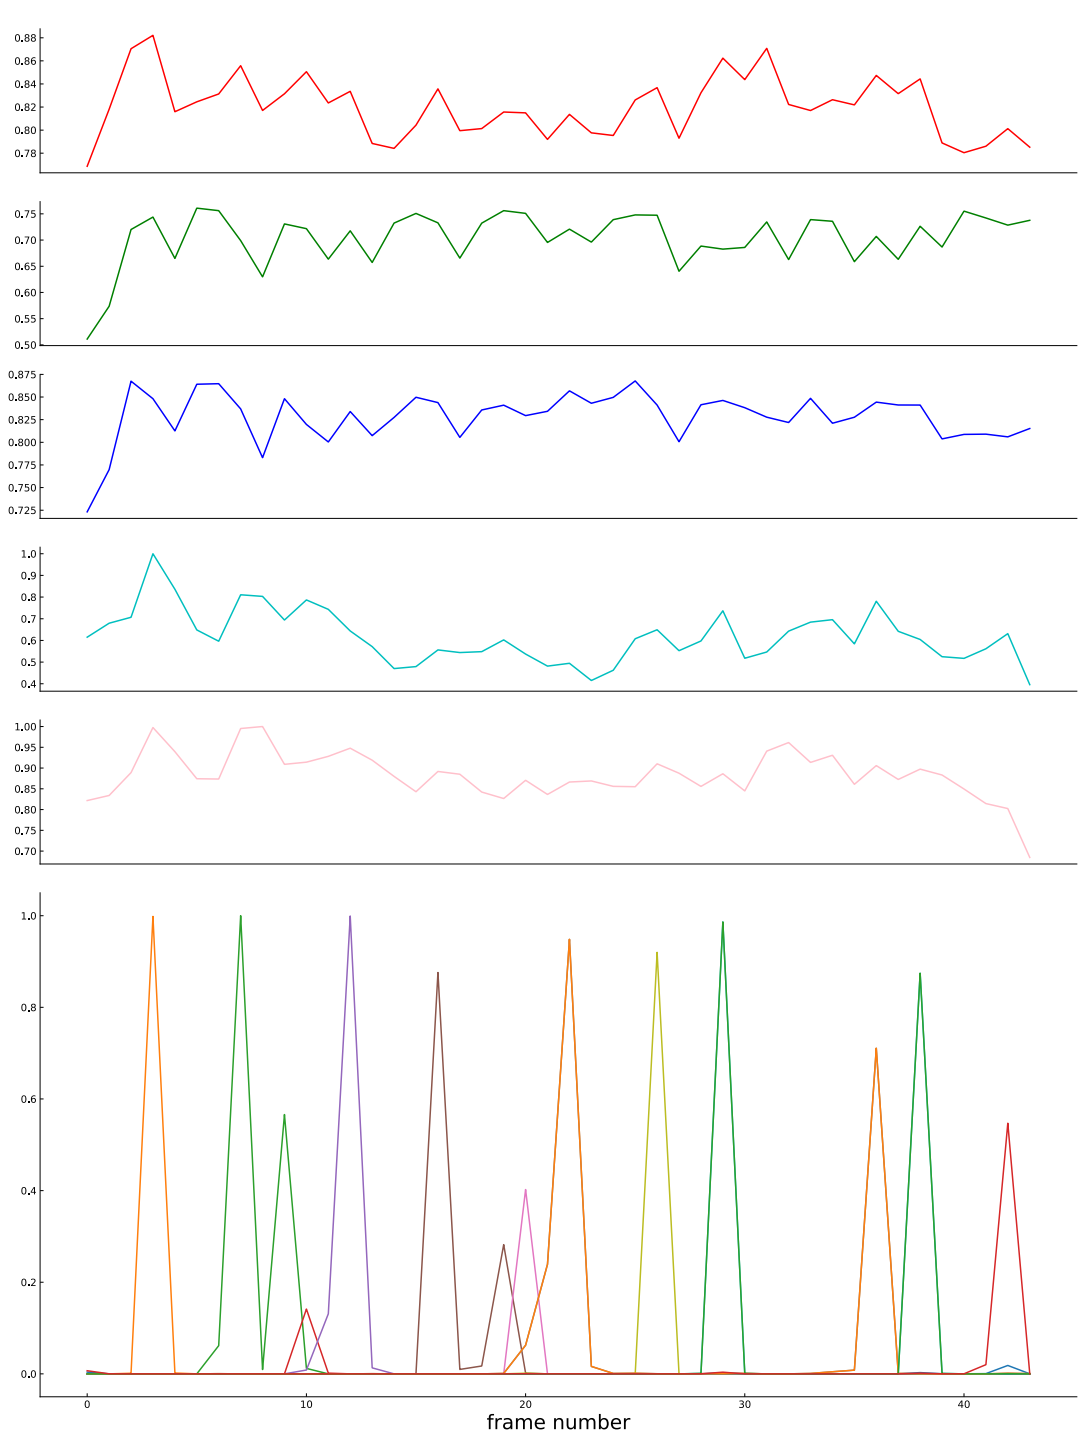

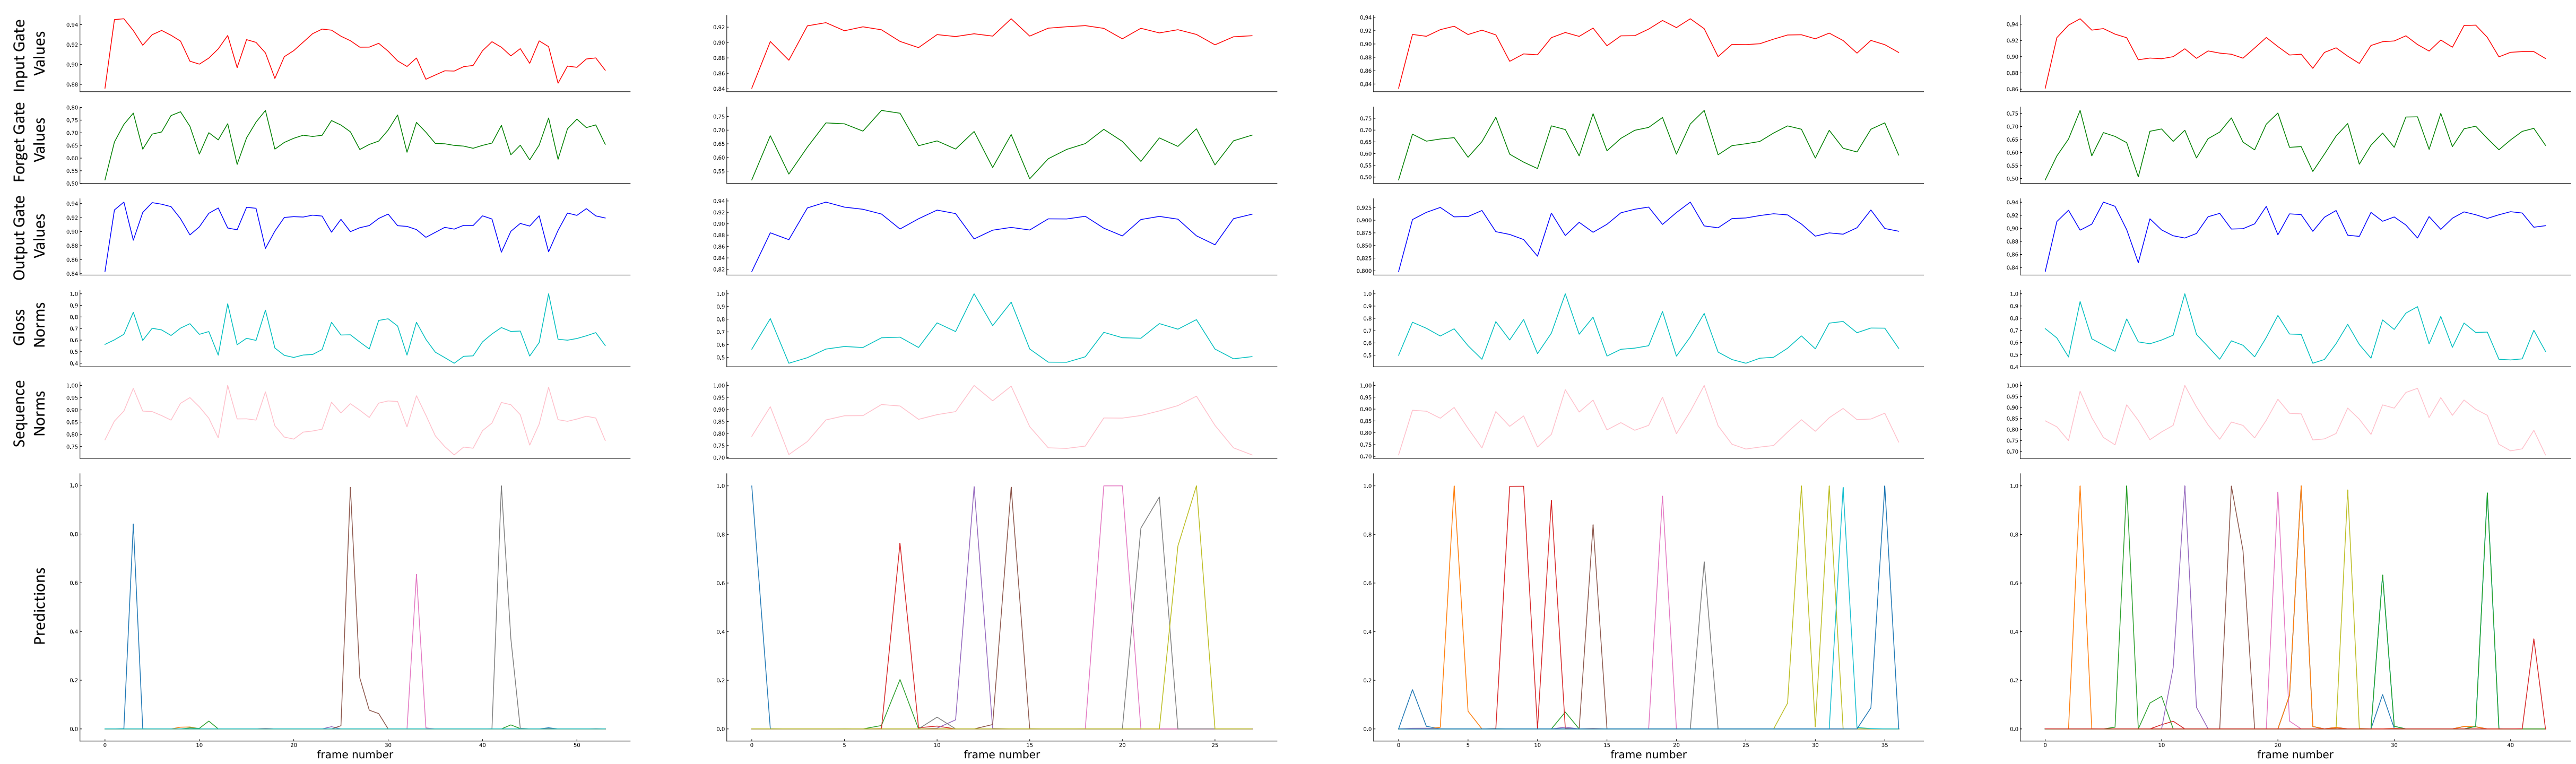

Supplement: Supplementary file 3 [file supp_figure11_norm_vis.pdf]
